# Supplementary material for: METR: Image Watermarking with Large Number of Unique Messages
Source: arXiv:2408.08340 source file (2024-08-15)
Supplement: Supplementary file 1 [file Appendix.tex]

% \begin{figure}[H]
% \label{fig:grid-search-changed-vae}
%     \centering
%     \includegraphics[width=0.3\textwidth]{test_pic.png}
%     \caption{
%     Grid search for METR with fine-tuned VAE decoder
%     }
% \end{figure}

% \begin{figure}[H]
% \centering
%     \begin{subfigure}[htp]{0.49\textwidth}
%         \centering
%         \includegraphics[width=0.99\linewidth]{images/graphs/grid_search/bit_acc_grid_default.png}
%         \subcaption{Bit accuracy}
%         \vspace{0.1\textwidth}
%     \end{subfigure}
%     \hfill
%     \begin{subfigure}[htp]{0.48\textwidth}
%         \centering
%         \includegraphics[width=0.99\linewidth]{images/graphs/grid_search/word_acc_grid_default.png}
%         \subcaption{Word accuracy}
%         \vspace{0.1\textwidth}
%     \end{subfigure}
%     \begin{subfigure}[htp]{0.48\textwidth}
%         \centering
%         \includegraphics[width=0.99\linewidth]{images/graphs/grid_search/det_resol_grid_default.png}
%         \subcaption{Detection resolution}
%         \vspace{0.1\textwidth}
%     \end{subfigure}
    
%     \vspace{0.025\textwidth}
    
%     \caption{
%     Grid search for METR with default VAE decoder. Detection metrics
%     }
%     \label{app:grid-search-default-vae}
    
% \end{figure}

% \newpage

% \begin{figure}[H]
% \centering
%     \begin{subfigure}[htp]{0.48\textwidth}
%         \centering
%         \includegraphics[width=0.99\linewidth]{images/graphs/grid_search/fid_gen_grid_default.png}
%         \subcaption{FID gen}
%         \vspace{0.1\textwidth}
%     \end{subfigure}
%     \hfill
%     \begin{subfigure}[htp]{0.48\textwidth}
%         \centering
%         \includegraphics[width=0.99\linewidth]{images/graphs/grid_search/fid_gt_grid_default.png}
%         \subcaption{FID gt}
        
%     \end{subfigure}
%     \vspace{0.025\textwidth}

%     \begin{subfigure}[htp]{0.48\textwidth}
%     \centering
%     \includegraphics[width=0.99\linewidth]{images/graphs/grid_search/w_clip_grid_default.png}
%     \subcaption{CLIP similarity}
%     \end{subfigure}

%     \vspace{0.025\textwidth}
    
%     \caption{
%     Grid search for METR with default VAE decoder. Image quality metrics. FID computation was made only on 500 images from MSCOCO
%     }
%     \label{app:grid-search-default-vae}
    
% \end{figure}


% \newpage

% \begin{figure}[ht]
% \centering
%     \begin{subfigure}[htp]{0.24\textwidth}
%         \centering
%         \includegraphics[width=0.99\linewidth]{images/graphs/detect_diff_treering_metr.png}
%         \subcaption{Diffusion attack on Tree-Ring}
%         \vspace{0.06\textwidth}
%     \end{subfigure}%
%     \begin{subfigure}[htp]{0.24\textwidth}
%         \centering
%         \includegraphics[width=0.99\linewidth]{images/graphs/detect_diff_metr.png}
%         \subcaption{Diffusion attack on METR}
%         \vspace{0.06\textwidth}
%     \end{subfigure}
%     \begin{subfigure}[htp]{0.24\textwidth}
%         \centering
%         \includegraphics[width=0.99\linewidth]{images/graphs/detect_vae_treering.png}
%         \subcaption{VAE~\cite{vae2018_attack} attack on Tree-Ring}
%         \vspace{0.035\textwidth}
%     \end{subfigure}%
%     \begin{subfigure}[htp]{0.24\textwidth}
%         \centering
%         \includegraphics[width=0.99\linewidth]{images/graphs/detect_vae_metr.png}
%         \subcaption{VAE~\cite{vae2018_attack} attack on METR}
%     \end{subfigure}
% \vspace{0.01\textwidth}
% \caption{Detection metrics for Tree-Ring and METR with Diffusion and VAE~\cite{vae2018_attack} attacks. Bit acc and Word acc are computed for METR with $S=100,~r=10$. Tree-Ring is not able to encrypt message, only detection metrics are shown.}
% \vspace{0.03\textwidth}
% \label{fig:}
% \end{figure}

% \caption{Diffusion attacks on Tree-Ring and METR. (a)~Tree-Ring is not able to encrypt message, only detection metrics are shown (b)~Bit acc and Word acc are computed for METR with $S=100,~r=10$.}
